# Supplementary material for: Adaptive Bidirectional Displacement for Semi-Supervised Medical Image Segmentation
Source: arXiv:2405.00378 source file (2024-05-01)
Supplement: Supplementary file 1 [file X_suppl.tex]

% \clearpage
% \setcounter{page}{1}
% \maketitlesupplementary

% \section{Clarify Uncontrolled Regions}
% ``uncontrolled regions" denote areas with relatively low confidence in predictions. We use predictions to evaluate whether the region is suitable to learn for the model.

\section{More Analysis}
\subsection{Different Displacement Strategies}
The original Tab. 4 shows the various displacement strategies in the ABD-R module. The ``Random" yield the worst results due to the uncertainty of this random displacement greatly increases the uncontrollability. While ``Reliable" exhibits a 0.2\% improvement in DSC compared to the ``Same" strategy, it theoretically effectively removes uncontrolled regions and displaces them with semantically similar information. Here, uncontrolled regions denote areas with relatively low confidence in predictions. We use predictions to evaluate whether the region is suitable to learn for the model. Although there are limited differences among the various displacement strategies in Tab. 4, our primary objective in the ABD-R module is to suppress uncontrollable regions to enhance model stability. It is only when the ABD-R and ABD-I modules are combined that their full potential can be realized.

\section{More Experimental Results}
\subsection{The Influence of Mixed Perturbation}
Fig.~\ref{fig1} indicates that involving additional input perturbation to Cross Pseudo Supervision (CPS)~\cite{chen2021semi} may lead to misclassifications, including erroneously recognizing background as foreground and incorrectly identifying foreground as background. 

\begin{figure}[!t]
\centering
\includegraphics[width=0.9\columnwidth]{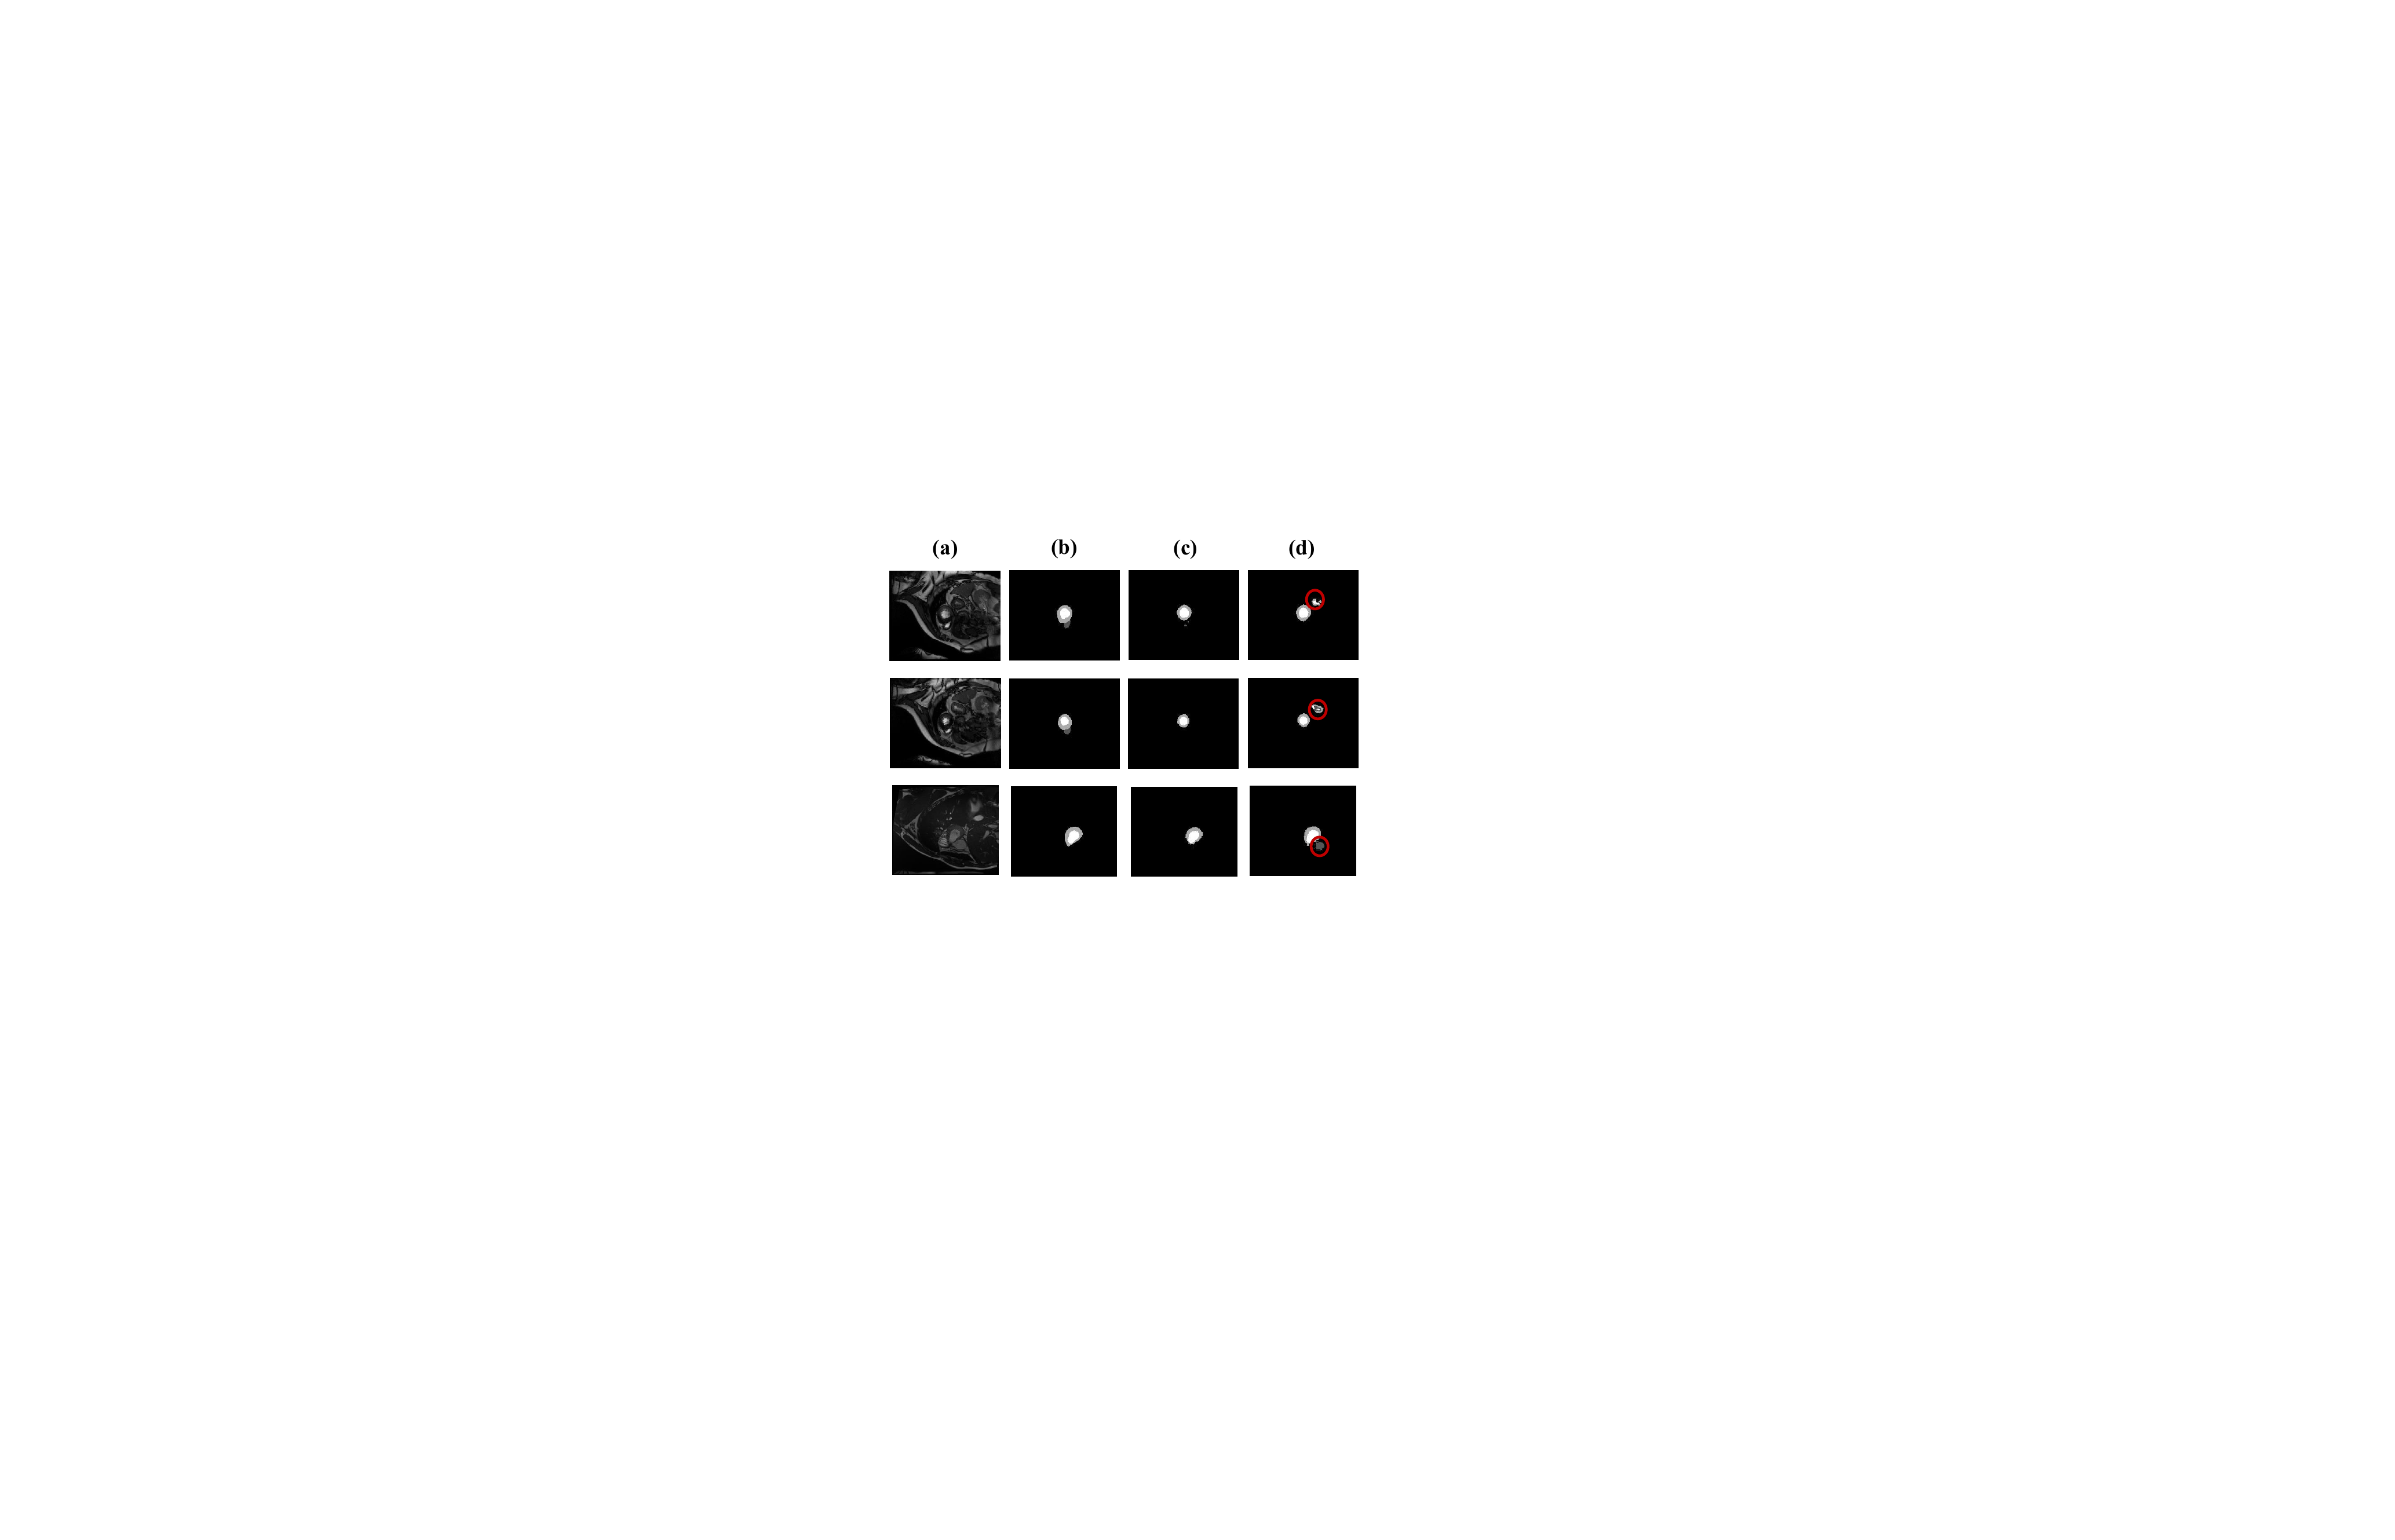}
\caption{ (a) Inputs; (b) Labels; (c) CPS prediction results; (d) Prediction results after adding input perturbation. The first two lines represent the prediction results of $f\left(\theta_1\right)$, while the last line represents the prediction results of $f\left(\theta_2\right)$. The areas highlighted by the red circles indicate regions of misclassification.}
\label{fig1}
\end{figure}

\begin{table*}[t]
\centering
\caption{Detailed Comparison on ACDC dataset}\label{tab:ACDC}
\resizebox{\textwidth}{!}{$
\begin{tabular}{c|cc|cc|cc|cc|cc}
\hline
\multirow{2}{*}{Method} & \multicolumn{2}{c|}{Scans used} & \multicolumn{2}{c|}{RV} & \multicolumn{2}{c|}{Myo} & \multicolumn{2}{c|}{LV} & \multicolumn{2}{c}{Avg}\\
\cline{2-11}
& Labeled & Unlabeled & DSC$\uparrow$ & 95HD$\downarrow$ & DSC$\uparrow$ & 95HD$\downarrow$ & DSC$\uparrow$ & 95HD$\downarrow$ & DSC$\uparrow$ & 95HD$\downarrow$\\
\hline
Cross Teaching & \multirow{3}{*}{3(5\%)} & \multirow{3}{*}{67(95\%)} & 57.70 & 21.4 & 62.80 & 11.5 & 76.30 & 15.7 & 65.60 & 16.2 \\
\textbf{Ours}-ABD (Cross Teaching) & & & 84.67 & 2.67 & 83.65 & 3.59 & 90.73 & 6.11 & 86.35 & 4.12 \\
\textbf{Ours}-ABD (BCP) & & & \textbf{88.69} & \textbf{1.46} & \textbf{85.78} & \textbf{1.99} & \textbf{92.42} & \textbf{1.27} & \textbf{88.96} & \textbf{1.57} \\
\hline
Cross Teaching & \multirow{3}{*}{7(10\%)} & \multirow{3}{*}{63(90\%)} & 84.80 & 7.80 & 84.40 & 6.90 & 90.10 & 11.20 & 86.40 & 8.60 \\
\textbf{Ours}-ABD (Cross Teaching) & & & 87.87 & 5.42 & 85.92 & 3.12 & 91.83 & 6.64 & 88.52 & 5.06 \\
\textbf{Ours}-ABD (BCP) & & & \textbf{89.47} & \textbf{1.27} & \textbf{86.70} & \textbf{1.22} & \textbf{93.25} & \textbf{1.88} & \textbf{89.81} & \textbf{1.46} \\
\hline
\end{tabular}%
$}
\end{table*}

\begin{figure*}[!t]
\centering
\includegraphics[width=1.0\textwidth]{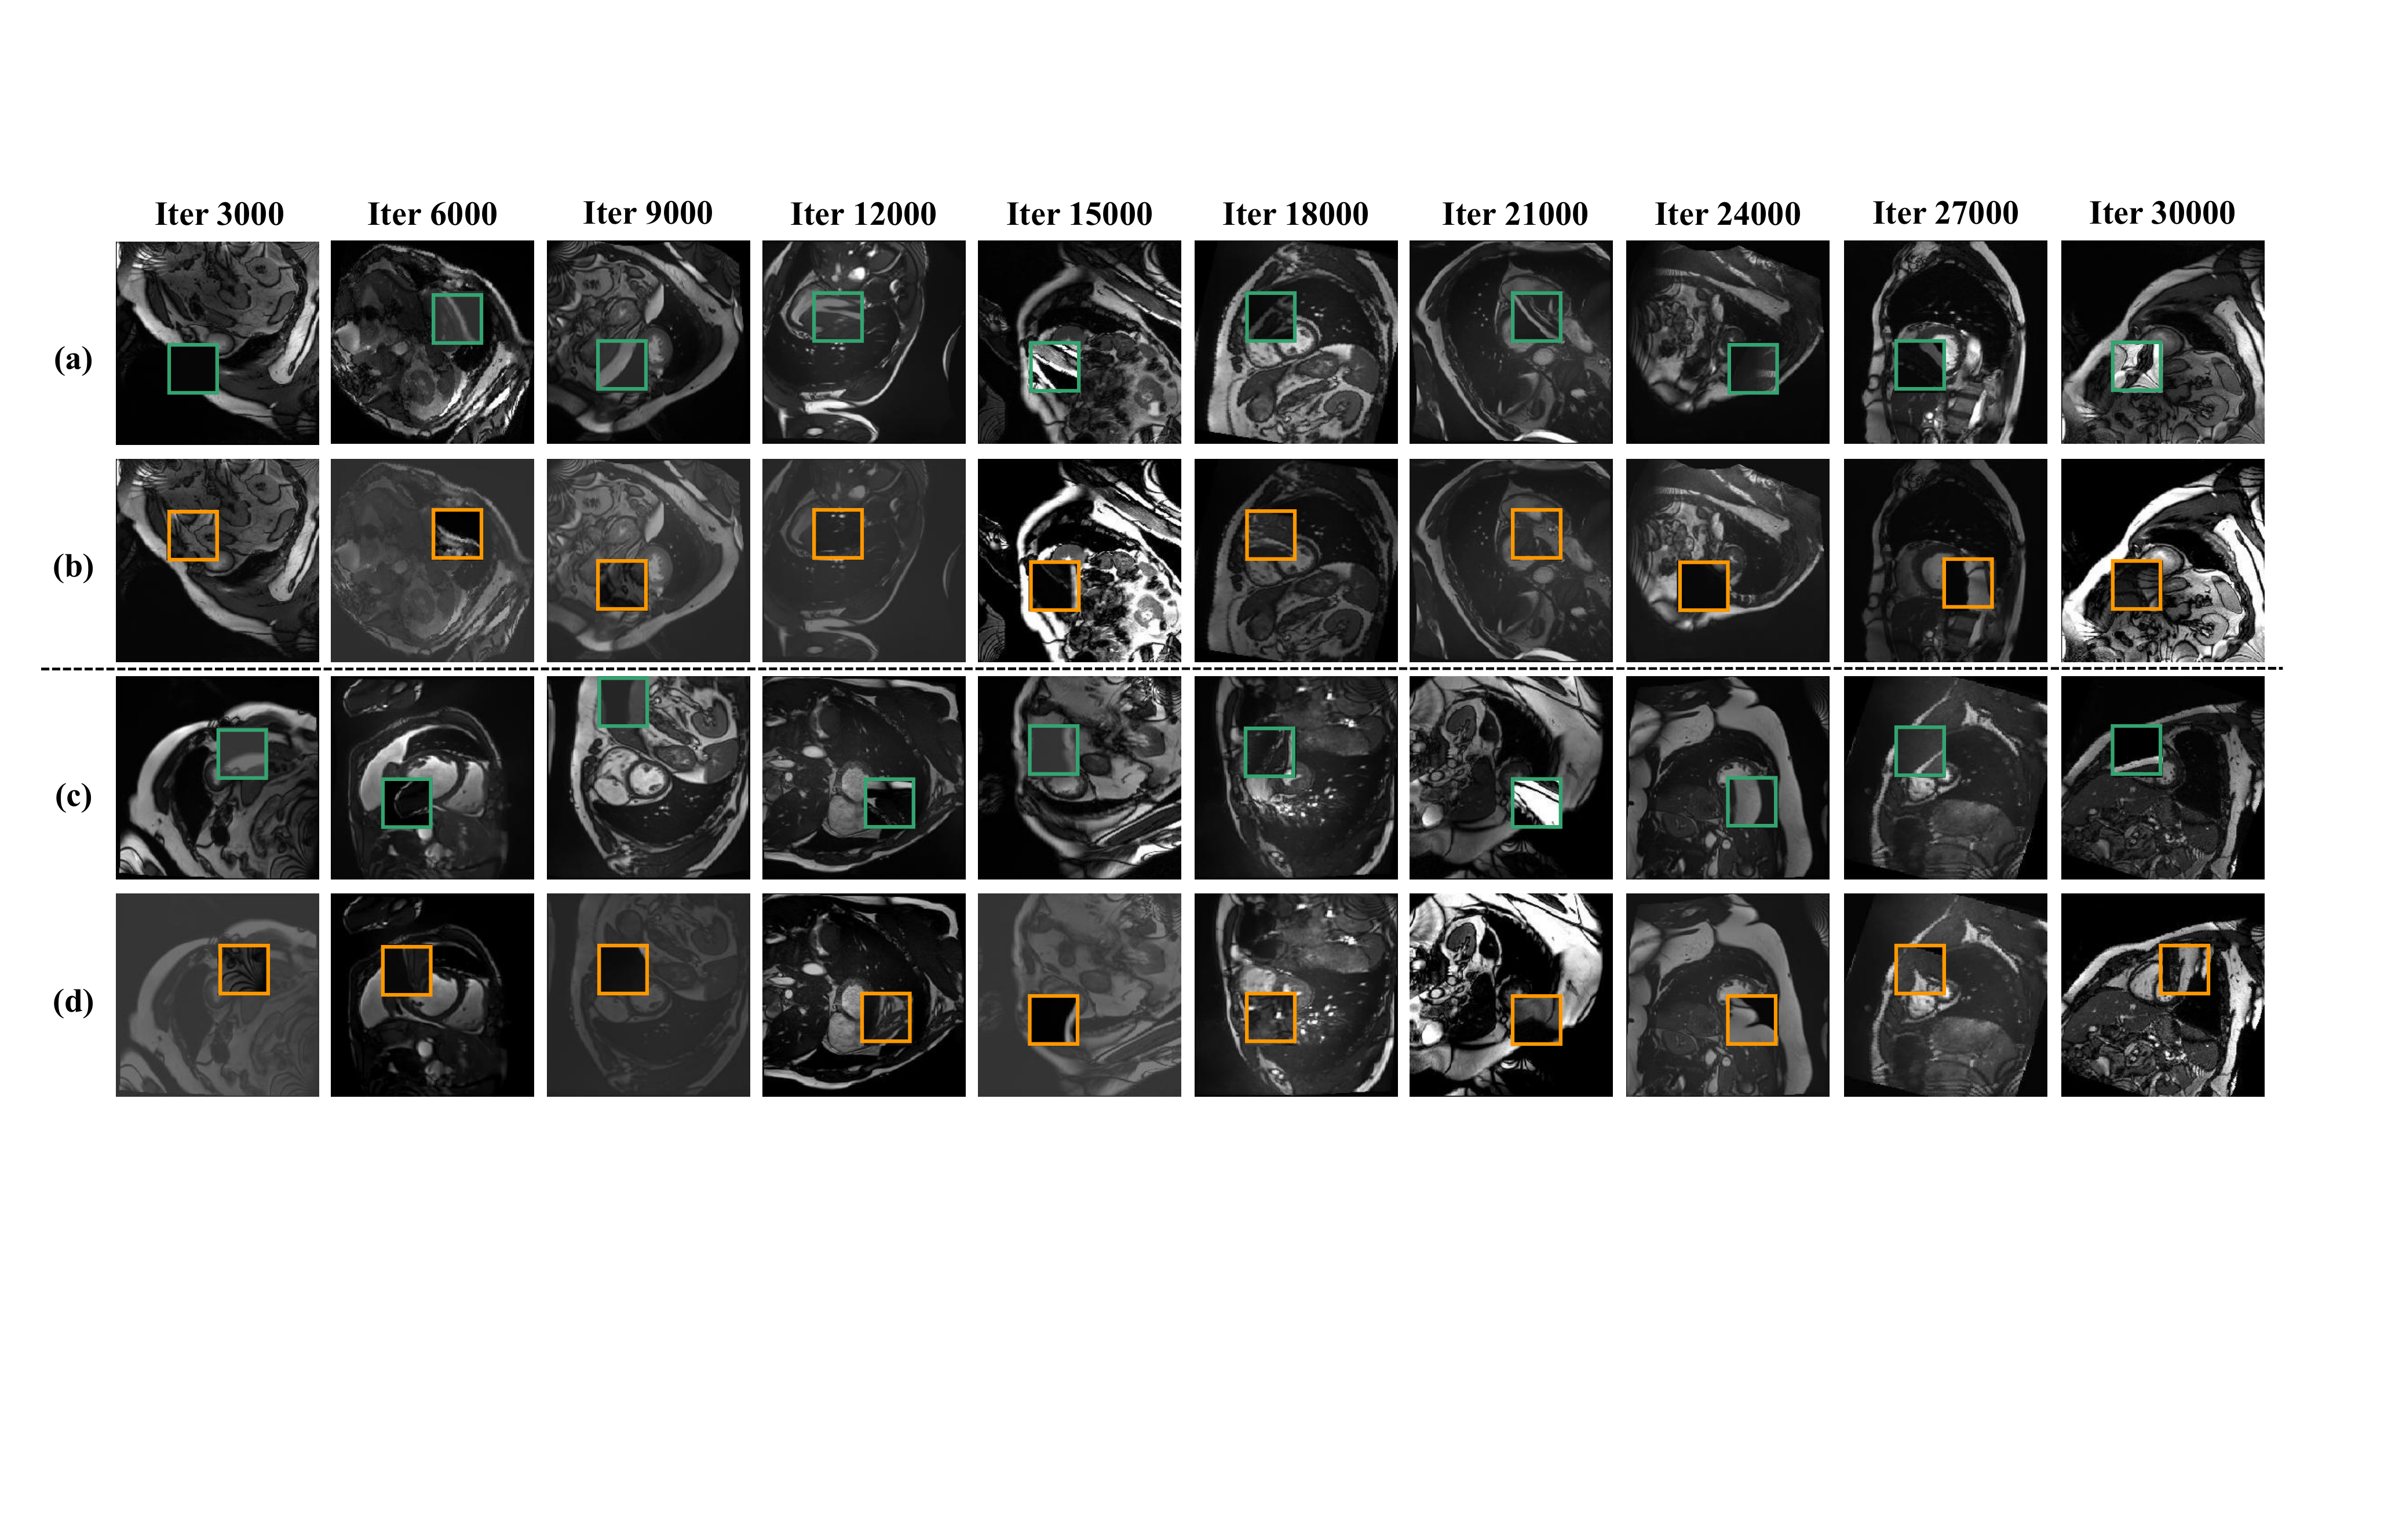} % Reduce the figure size so that it is slightly narrower than the column.
\caption{Visualization of generated samples from ABD-R with unlabeled data. The generated sample pairs (a) and (b) are specifically derived from weakly and strongly augmented images. The green box in (a) represents the final selected semantic derived from (b). The orange box in (b) represents the final selected semantic derived from (a). Samples in (c) and (d) are generated in the same way as above.} \label{ABD-R}
\end{figure*}

\begin{figure*}[!t]
\centering
\includegraphics[width=1.0\textwidth]{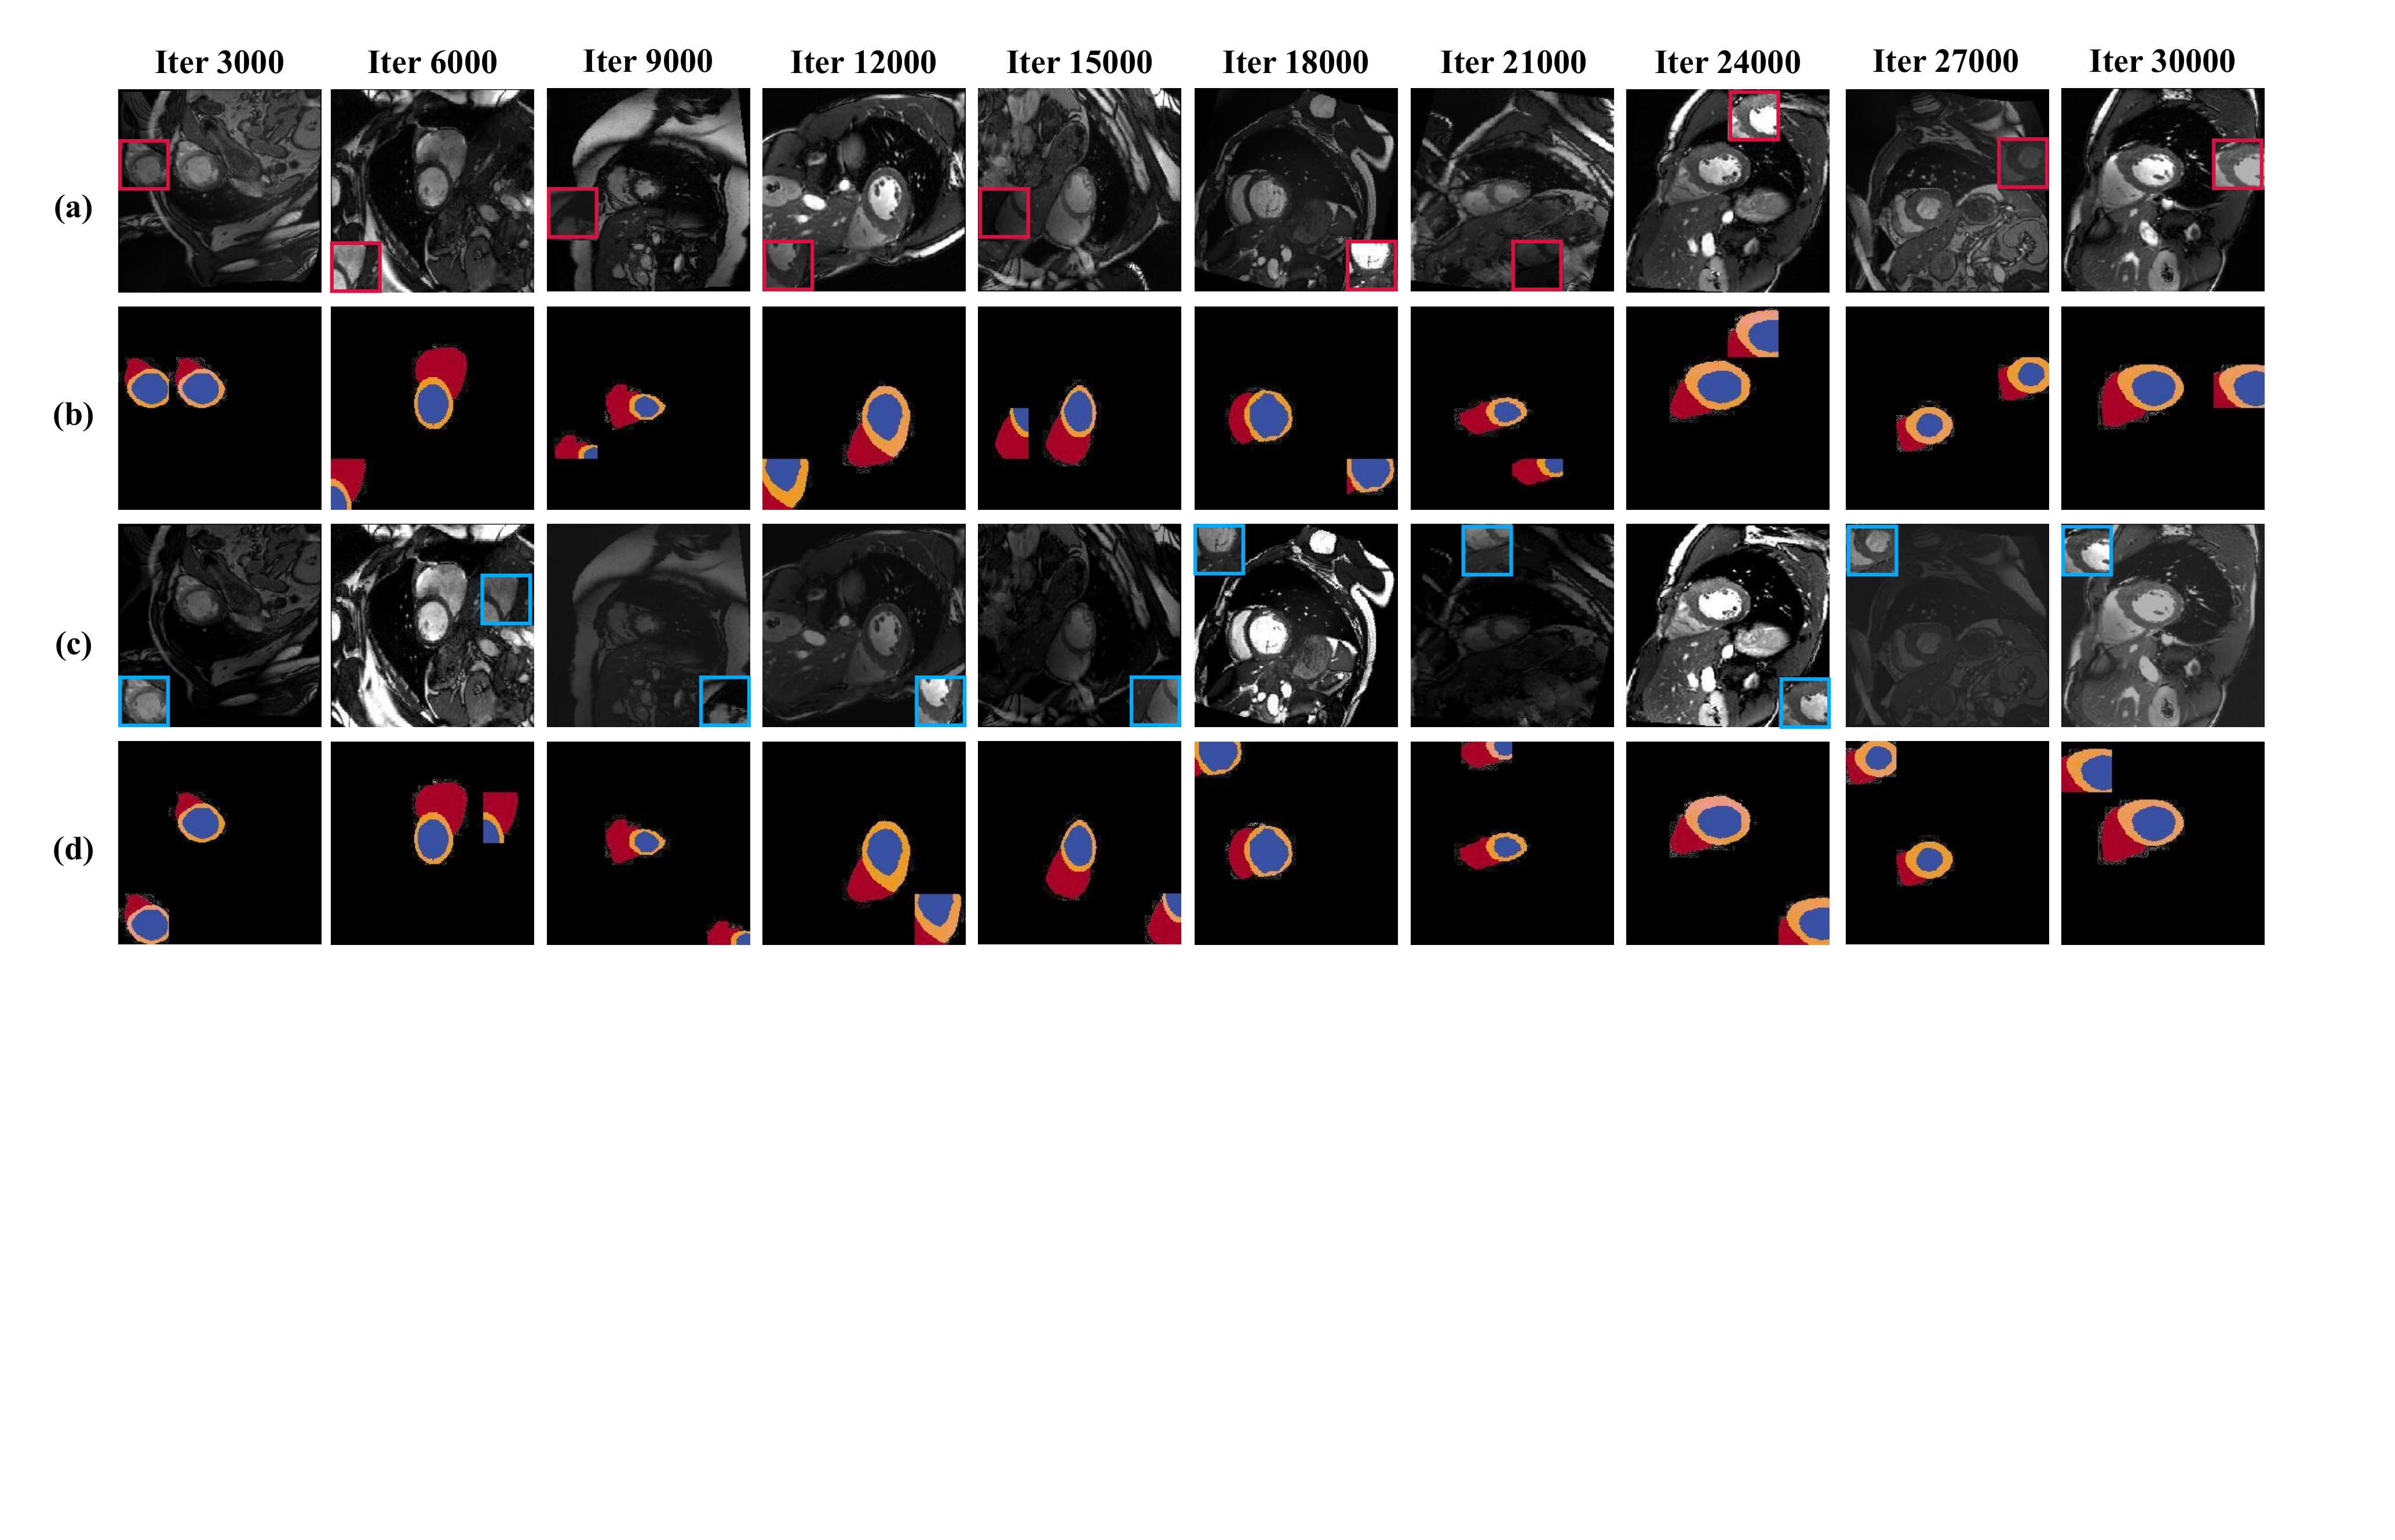} % Reduce the figure size so that it is slightly narrower than the column.
\caption{Visualization of generated samples and labels from ABD-I with labeled data. (a) and (c) are the generated samples based on weakly and strongly augmented images. The red box in (a) represents the lowest confidence semantic derived from (c). (b) The generated labels correspond to the samples from (a). The blue box in (c) represents the lowest confidence semantic derived from (a). (d) The generated labels correspond to the samples from (c)} \label{ABD-I}
\end{figure*}

\subsection{Detailed Comparison on ACDC}
In Tab.~\ref{tab:ACDC}, we show the detailed comparison between our approach and Cross teaching on ACDC dataset. It can be seen that our approach, \ie, \textbf{Ours}-ABD (Cross Teaching~\cite{luo2022semi}) significantly improves the performance of the baseline (Cross Teaching). After introducing our approach to the more powerful approach BCP~\cite{bai2023bidirectional}, it reaches a new state-of-the-art result.

\subsection{Visualization of Adaptive Bidirectional Displacement}
Fig.~\ref{ABD-R} shows the generated samples of the Adaptive Bidirectional Displacement with Reliable Confidence (ABD-R) under different iterations. It can be observed that, in different iterations, ABD-R replaces the lowest confident regions with the final regions selected with high confidence sourced from another augmented image. As a result, the generated samples have compensated semantics, ensuring the reliability of consistency learning. Fig.~\ref{ABD-I} visualizes the generated samples of the Adaptive Bidirectional Displacement with Inverse Confidence (ABD-I) under different iterations. Fig.~\ref{ABD-I} indicates that the newly generated samples contain more low confident semantics information compared to the original augmented image, those samples can empower the model to effectively learn from the potentially uncontrollable regions.

\subsection{Selection of Patch Number on ACDC and PROMISE12}
Tab.~\ref{tab:ACDC-size} demonstrates how different patch numbers impact the performance of the model on ACDC when only 5\% labeled data is used. We also add the ablation study of the patch number on PROMISE12 dataset in Tab.~\ref{tab:PROMISE12-size}. $K$ represents the number of patches in the image. It can be observed that selecting $K=16$ is the most appropriate choice in both cases, as both excessively large and small values of $K$ do not contribute significantly to learn meaningful semantics. If $K$ is too small, \eg, $K$ is $2$, suppose the $2$nd region will be replaced by the $1$st region from the other image, it will produce a new sample formed by two ``$1$st region", totally lost information in the $2$nd region. The opposite situation occurs if $K$ is too large.

\begin{table}[!t]
\caption{Ablation study of patch number $K$ with 5\% labeled data.} \label{tab:ACDC-size}
\centering
\begin{tabular}
{c|cccc}
\hline
$K$ & DSC$\uparrow$ & Jaccard$\uparrow$ & 95HD$\downarrow$ & ASD$\downarrow$ \\
\hline
4 & 85.31 & 75.35 & 4.32 & 1.47 \\
16 & \textbf{86.35} & \textbf{76.73} & \textbf{4.12} & \textbf{1.22} \\
64 & 85.56 & 75.64 & 4.50 & 1.35 \\
\hline
\end{tabular}
\end{table}

\begin{table}[!t]
\caption{Ablation study of patch number $K$ on PROMISE12.} \label{tab:PROMISE12-size}
\centering
% \setlength{\extrarowheight}{0.8pt}
% \resizebox{\columnwidth}{!}{$
\begin{tabular}
{c|cccc}
\hline
$K$ & DSC$\uparrow$ & Jaccard$\uparrow$ & 95HD$\downarrow$ & ASD $\downarrow$ \\
\hline
4  & 78.20 & 64.58 & 3.81 & 1.63  \\
16 & \textbf{82.06} & \textbf{69.94} & \textbf{3.02} & \textbf{1.33} \\
64 & 78.85 & 65.45 & 5.59 & 2.25 \\ 
\hline
\end{tabular}
% $}
\end{table}

\subsection{Selection of Top-n Highest Confidence Patches on ACDC}
Tab.~\ref{tab:top} demonstrates how different numbers of top highest confidence patches impact the performance of the model when only 10\% labeled data is used. $n$ represents the top $n$ highest confidence levels in the image. It can be observed that $n=4$ generates better performance than others. When $n$ is too small, the final regions selected with high confidence may not closely align with the original semantics. Conversely, if $n$ is too large, it may result in the final selection of regions with relatively low confidence, leading to uncontrollable outcomes.

\begin{table}[t]
\centering
\caption{Ablation study of top-$n$ highest confidence patches with 10\% labeled data.} \label{tab:top}
\begin{tabular}
{c|cccc}
\hline
$n$ & DSC$\uparrow$ & Jaccard$\uparrow$ & 95HD$\downarrow$ & ASD$\downarrow$ \\
\hline
2 & 87.90 & 79.13 & 5.53 & 1.70 \\
4 & \textbf{88.52} & \textbf{79.97} & \textbf{5.06} & \textbf{1.43} \\
8 & 87.94 & 79.10 & 6.32 & 1.80 \\
\hline
\end{tabular}
\end{table}
